# Supplementary material for: A unified framework of non-local parametric methods for image denoising
Source: arXiv:2402.13816 source file (2024-02-21)
Supplement: Supplementary file 1 [file algo.tex]

\section{A sequential coordinate descent algorithm for quadratic programming under conical and convex constraints}

The following sequential coordinate descent algorithm computes an approximation of the minimizer of \begin{equation}
    q(\theta) =\frac{1}{2} \theta^\top Q \theta + c^\top \theta
\end{equation}
\noindent with $Q \in \mathbb{R}^{k \times k}$ and $c \in \mathbb{R}^{k}$ under conical (\textit{i.e} $\theta \succeq 0$) or convex (\textit{i.e} $\mathbf{1}_k^\top \theta = 1$ and $\theta \succeq 0$) constraints. It is 
employed in practice for fast approximation  of the columns of $\hat{\Theta}_{cnl}$ and  $\hat{\Theta}_{cvx}$, respectively, in NL-Ridge algorithm. \Cref{SCD_conical_convex} details the descent procedure in both cases. Note that the proposed algorithm produces, by construction, a sequence of feasible iterates $\theta^{(0)}, \ldots, \theta^{(T)}$ such that $q(\theta^{(0)})  \geq \ldots \geq q(\theta^{(T)})$, where $q$ denotes the objective function.

\begin{algorithm}
\caption{Sequential coordinate descent for minimizing the quadratic program $q(\theta) =\frac{1}{2} \theta^\top Q \theta + c^\top \theta$ under conical (\textit{i.e} $\theta \succeq 0$) or convex (\textit{i.e} $\mathbf{1}_k^\top \theta = 1$ and $\theta \succeq 0$) constraints.}
\label{SCD_conical_convex}
\begin{algorithmic}
\STATE{Input: Number of iterations $T$}
\STATE{Start with an initial estimate  $\theta^{(0)} = \mathbf{1}_k / k$}
\FOR{$t = 1, \ldots, T$}
    \STATE{$\theta^{(t)}\leftarrow \theta^{(t-1)} $}
    \FOR{$j = 1, \ldots, k$}
        \STATE{Choose descent direction $d_j = \left\{
    \begin{array}{ll}
        e_j & \small \textit{(conical constraint)}\\
        e_j - e_{j'}  &  \small \textit{(convex constraint)}
    \end{array}
\right.$ with $j' \in \{1, \ldots, k  \} \setminus \{j \}$  chosen at random}

\STATE{Solve the unidimensional problem:}

$$\begin{aligned}
       \alpha^\ast &= \mathop{\arg \min}\limits_{\substack{\alpha \in \mathbb{R}\; s.t. \\ \theta^{(t)} + \alpha d_j \succeq 0}} q(\theta^{(t)} + \alpha d_j) \\
    &= 
  \left\{\begin{array}{ll}
        \max(-\frac{\theta^{(t) \top } Q_{\cdot,j}  + c_j}{Q_{j,j}} ,-\theta^{(t)}_j)  & \textit{(conical constraint)}\\
        \min(\max(-\frac{\theta^{(t) \top} (Q_{\cdot, j} -  Q_{\cdot, j'})    + c_j - c_{j'}}{Q_{j,j}- 2 Q_{j,j'}+Q_{j',j'}}, -\theta^{(t)}_j), \theta^{(t)}_{j'}) &  \textit{(convex constraint)}
    \end{array}
\right.\end{aligned}$$ 
\STATE{Update $\theta^{(t)}$: $$\theta^{(t)} \leftarrow \theta^{(t)} + \alpha^\ast d_j$$}
\ENDFOR
\ENDFOR
\RETURN{$\theta^{(T)}$}
\end{algorithmic}
\end{algorithm}
